# Supplementary material for: Isomeric excitation of ^{229}\mathrm{Th} via scanning tunneling microscope
Source: arXiv:2310.06352 source file (2023-10-10)
Supplement: Supplementary file 1 [file supplementary.pdf]

# Supplementary Material for “Isomeric excitation of $^{229}\text{Th}$ via scanning tunneling microscope”

Xue Zhang, Tao Li, Xu Wang,\* and Hui Dong†  
Graduate School of China Academy of Engineering Physics,  
No. 10 Xibeiwang East Road, Haidian District, Beijing, 100193, China

The current Supplementary Material provides detailed derivations of the results in the main text, and supporting discussions.

## CONTENTS

|                                                                  |   |
|------------------------------------------------------------------|---|
| I. Electron wave functions                                       | 1 |
| II. Electron transition matrix element $\Xi_{fi}^{\mathcal{T}l}$ | 1 |
| III. Numeral Calculations of Transition probability              | 2 |
| IV. The Applied Positive Bias Voltage                            | 3 |
| V. The impact of the position of the tip                         | 4 |
| References                                                       | 4 |

## I. ELECTRON WAVE FUNCTIONS

In the current discussion, the tip apex is considered as a metallic sphere with its wave function in the vacuum region as an asymptotic spherical shape

$$\phi_k(\mathbf{r}) = A_k \frac{\exp[-\kappa_k(|\mathbf{r} - \mathbf{a}| - R_t)]}{\kappa_k |\mathbf{r} - \mathbf{a}|}, \quad (1)$$

where  $\mathbf{a} = (0, 0, d + R_t)$  is the position of the center of the tip and  $R_t$  is the radius of curvature of the tip.  $\kappa_k = \sqrt{-2m_e \xi_k}/\hbar$  is the attenuation factor and  $A_k$  is the normalization coefficient. We choose the area below the needle tip as the integration area in the later calculation. Assuming the center of tip is the origin, i.e.  $\mathbf{a}=0$ , we get normalization coefficient  $A_k = \sqrt{\kappa_k^3/\pi}$  according to normalization conditions  $\int d\mathbf{r} |\phi_k(\mathbf{r})|^2 = 1$ . This wave function is typical known as the s wave, which is the simplest case for the tip [1]. The surface wave function of the bare metal substrate in the vacuum region takes the form [2, 3]

$$\varphi_n(\mathbf{r}) = B_n \exp(-\kappa_n |z|), \quad (2)$$

where  $\kappa_n = \sqrt{-2m_e E_n}$  is the attenuation factor and  $B_n$  is the normalization coefficient. Since the wave function of metal surface waves only exists in the upper half plane (i.e.  $z > 0$ ), we obtain  $B_n = \sqrt{2\kappa_n}$  according to normalization conditions  $\int d\mathbf{r} |\varphi_n(\mathbf{r})|^2 = 1$ . Experiments have shown that the insulating layer on the metal surface does not change the lineshape of the substrate-photon-emission spectrum but only reduces its intensity[4].

## II. ELECTRON TRANSITION MATRIX ELEMENT $\Xi_{fi}^{\mathcal{T}l}$

We get the current  $\mathbf{j}_{fi}(\mathbf{r})$  of the electron tunneling from the substrate to the tip as

$$\mathbf{j}_{fi}(\mathbf{r}) = -e \frac{i\hbar}{2m_e} (\phi_k \nabla \varphi_n - \varphi_n \nabla \phi_k). \quad (3)$$

---

\* xwang@gscaep.ac.cn

† hdong@gscaep.ac.cn

With the expression of  $\mathcal{B}_{lm}^E(kr)$  in the main paper, we calculate electron transition matrix element  $\Xi_{fi}^{Tl}$

$$\Xi_{fi}^{El} = \frac{-i}{k\sqrt{l(l+1)}} \int d\mathbf{r} \mathbf{j}_{fi}(\mathbf{r}) \cdot \nabla \times \mathbf{L} h_l^{(1)}(kr) Y_{lm}(\hat{\mathbf{r}}), \quad (4)$$

$$\Xi_{fi}^{Ml} = \frac{1}{\sqrt{l(l+1)}} \int d\mathbf{r} \mathbf{j}_{fi}(\mathbf{r}) \cdot \mathbf{L} h_l^{(1)}(kr) Y_{lm}(\hat{\mathbf{r}}), \quad (5)$$

where  $k\hbar c = E_0 - E_1 = E_{eg}$  is the energy lost by tunneling electrons, corresponding to the energy gap  $E_{eg}$  between the ground state and the excited state of the nucleus. With the identity  $\nabla \times \mathbf{L} f_l(kr) Y_{lm}(\hat{\mathbf{r}}) = i\nabla \left( \frac{\partial}{\partial r} (r f_l(kr)) Y_{lm} \right) + ik^2 \mathbf{r} f_l(kr) Y_{lm}(\hat{\mathbf{r}})$  and the flow conservation equation  $\nabla \cdot \mathbf{j}_{fi} = ikce\phi_k\varphi_n$ , we get

$$\begin{aligned} \Xi_{fi}^{El} &= \frac{ic}{\sqrt{l(l+1)}} \int d\mathbf{r} \rho_{fi} \frac{\partial}{\partial r} \left( r h_l^{(1)}(kr) \right) Y_{lm}(\hat{\mathbf{r}}) \\ &\quad + \frac{k}{\sqrt{l(l+1)}} \int d\mathbf{r} \mathbf{j}_{fi}(\mathbf{r}) \cdot \mathbf{r} h_l^{(1)}(kr) Y_{lm}(\hat{\mathbf{r}}), \end{aligned} \quad (6)$$

where  $\rho_{fi} = e\phi_k\varphi_n$  is a density-like function.

Using the spherical coordinate system for simplicity of expression, we obtain

$$\begin{aligned} \Xi_{fi}^{El} &= -\frac{icl}{\sqrt{l(l+1)}} \int d\mathbf{r} \phi_k \varphi_n h_l^{(1)}(kr) Y_{lm}(\hat{\mathbf{r}}) \\ &\quad + \frac{ick}{\sqrt{l(l+1)}} \int d\mathbf{r} r \phi_k \varphi_n h_{l-1}^{(1)}(kr) Y_{lm}(\hat{\mathbf{r}}) \\ &\quad + \frac{i\hbar}{2m_e} \frac{k}{\sqrt{l(l+1)}} \int d\mathbf{r} \kappa_n r \cos \theta \phi_k \varphi_n h_l^{(1)}(kr) Y_{lm}(\hat{\mathbf{r}}) \\ &\quad - \frac{i\hbar}{2m_e} \frac{k}{\sqrt{l(l+1)}} \int d\mathbf{r} r^2 \phi_k \varphi_n h_l^{(1)}(kr) Y_{lm}(\hat{\mathbf{r}}) \frac{1 + \kappa_k |\mathbf{r} - \mathbf{a}|}{|\mathbf{r} - \mathbf{a}|^2} \\ &\quad + \frac{i\hbar}{2m_e} \frac{k}{\sqrt{l(l+1)}} \int d\mathbf{r} kr \cos \theta \phi_k \varphi_n h_l^{(1)}(kr) Y_{lm}(\hat{\mathbf{r}}) \frac{1 + \kappa_k |\mathbf{r} - \mathbf{a}|}{|\mathbf{r} - \mathbf{a}|^2} \end{aligned} \quad (7)$$

and

$$\Xi_{fi}^{Ml} = \frac{e\kappa_n}{\sqrt{l(l+1)}} \frac{\hbar^2}{2m_e} \int d\mathbf{r} \phi_k \varphi_n \left[ \kappa_n + (R_t + d) \frac{1 + \kappa_k |\mathbf{r} - \mathbf{a}|}{|\mathbf{r} - \mathbf{a}|^2} \right] h_l^{(1)}(kr) \frac{\partial}{\partial \phi} Y_{lm}(\hat{\mathbf{r}}). \quad (8)$$

In our setup, the wave functions  $\phi_k(\mathbf{r})$  and  $\varphi_n(\mathbf{r})$  have no component of angle  $\phi$ , resulting the vanishing component  $\Xi_{fi}^{Ml} \propto \int d\phi \partial Y_{lm}(\hat{\mathbf{r}}) / \partial \phi = 0$ , due to  $\partial Y_{lm}(\hat{\mathbf{r}}) / \partial \phi \propto -ime^{-im\phi}$ .

### III. NUMERICAL CALCULATIONS OF TRANSITION PROBABILITY

In this study, we consider both the tip and substrate with the material of the silver (Ag). The density of states (DOS) of Ag is presented in Fig. 1, obtained from reference [5]. In the numerical calculation, we select a cylinder with the height  $d$  as the integration area in cylindrical coordinate system  $(r, \phi, z)$  and ensure that the integral converges when the radius of the cylinder is reached. For the integration of energy  $E_n$ , we choose the number (50) of energy intervals to ensure its convergence, and finally get the transition probability  $P$  of Fig. 2 in the main article.

Fig. 2 shows the transition probability as a function of tip radius  $R_t$  with different applied bias voltage  $V_b$ . For small bias voltages, non-monotonic curves differing from those in the main article emerge. This is attributed to the increasing overlap of wave functions between the tip and substrate as the tip radius  $R_t$  decreasing at a small bias voltage. The larger overlap facilitates electron tunneling between the tip and substrate, leading to an enhanced transition probability.

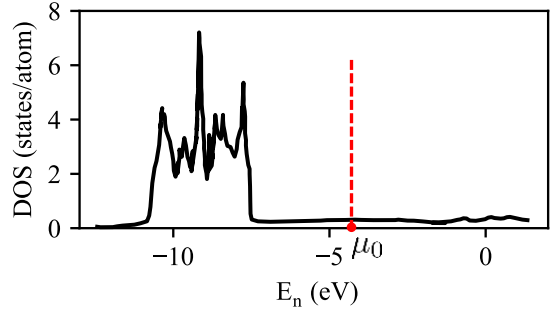

Figure 1. The density of states (DOS) of Ag.  $\mu_0 = -4.64\text{eV}$  is the fermi energy of Ag.

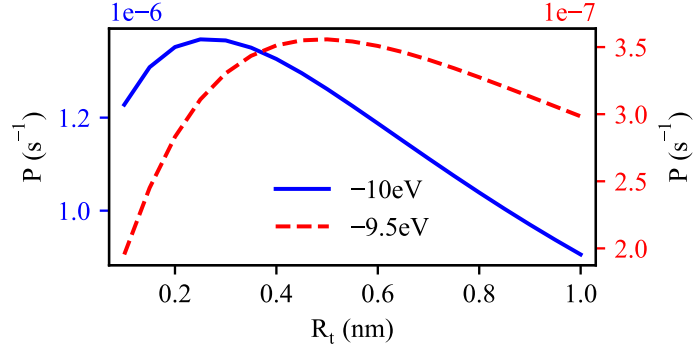

Figure 2. Transition probability  $P$  as a function of tip radius  $R_t$ . The distance  $d$  is fixed at  $0.5\text{nm}$  and the applied bias voltage  $V_b$  is set to  $-10\text{V}$  for blue solid line and  $-9.5\text{V}$  for red dashed line, respectively.

#### IV. THE APPLIED POSITIVE BIAS VOLTAGE

We sketched the design of a single Th atom STM in Fig. 3 with a applied positive bias voltage  $V_b$ . For positive bias, i.e.  $V_b > 0$ , the electron runs from the tip to the substrate (see Fig. 3(b)). The electron tunneling current is

$$\mathbf{j}_{fi}^+(\mathbf{r}) = e \frac{i\hbar}{2m_e} (\phi_k \nabla \varphi_n - \varphi_n \nabla \phi_k), \quad (9)$$

which is the inverse of that in negative bias, i.e.  $\mathbf{j}_{fi}^+(\mathbf{r}) = -\mathbf{j}_{fi}(\mathbf{r})$ . This causes a slight change in  $\Xi_{fi}^{El}$  in Eq. (7), but does not change its leading term. In conclusion, a variation in the applied bias electrode does not result in a alteration of the transition probability  $P$ .

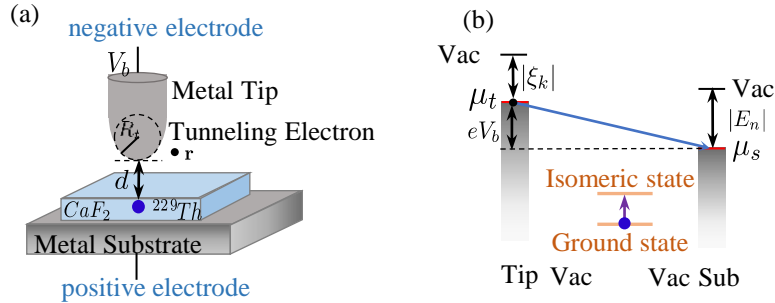

Figure 3. Schematic diagram of STM of a single  $^{229}\text{Th}$  with a applied positive bias voltage  $V_b$ . (b) The level diagram for inelastic electron scattering mechanism at bias voltage in (a). The symbols are the same as those in the main paper.

## V. THE IMPACT OF THE POSITION OF THE TIP

One of the advantages in the current scheme is the precise location of the tip to allow the focus of the tunneling electrons on one single  $^{229}\text{Th}$ . Here we consider that the impact of the tip position with a small displacement relative to the center of the atom in the case of negative bias voltage. We assume the position of the center of the tip  $\mathbf{a} = (a_x, a_y, d + R_t)$ . Using the same calculation method, we can get

$$\begin{aligned} \Xi_{fi}^{El} = & -\frac{eicl}{\sqrt{l(l+1)}} \int d\mathbf{r} \phi_k \varphi_n h_l^{(1)}(kr) Y_{lm}(\hat{\mathbf{r}}) \\ & + \frac{eick}{\sqrt{l(l+1)}} \int d\mathbf{r} \phi_k \varphi_n r h_{l-1}^{(1)}(kr) Y_{lm}(\hat{\mathbf{r}}) \\ & + \frac{ei\hbar}{2m_e} \frac{k}{\sqrt{l(l+1)}} \kappa_n \int d\mathbf{r} r \cos \theta \phi_k \varphi_n h_l^{(1)}(kr) Y_{lm}(\hat{\mathbf{r}}) \\ & - \frac{ei\hbar}{2m_e} \frac{k}{\sqrt{l(l+1)}} \int d\mathbf{r} [r^2 - r \cos \theta (R_t + d)] \phi_k \varphi_n h_l^{(1)}(kr) Y_{lm}(\hat{\mathbf{r}}) \frac{1 + \kappa_k |\mathbf{r} - \mathbf{a}|}{|\mathbf{r} - \mathbf{a}|^2} \\ & + \frac{ei\hbar}{2m_e} \frac{k}{\sqrt{l(l+1)}} \int d\mathbf{r} [r \sin \theta \cos \phi a_x + r \sin \theta \sin \phi a_y] \phi_k \varphi_n h_l^{(1)}(kr) Y_{lm}(\hat{\mathbf{r}}) \frac{1 + \kappa_k |\mathbf{r} - \mathbf{a}|}{|\mathbf{r} - \mathbf{a}|^2}. \end{aligned} \quad (10)$$

Since  $kr \ll 1$ , the first term is the leading term.

The electron matrix element  $\Xi_{fi}^{Ml}$  is nonzero in this case because the tip wave function depends on the angle  $\phi$ . We give the final expression of  $\Xi_{fi}^{Ml}$ ,

$$\begin{aligned} \Xi_{fi}^{Ml} = & \frac{e\kappa_n}{\sqrt{l(l+1)}} \frac{\hbar^2}{2m_e} \int d\mathbf{r} \phi_k \varphi_n h_l^{(1)}(kr) \frac{\partial}{\partial \phi} Y_{lm}(\hat{\mathbf{r}}) \\ & + \frac{e}{\sqrt{l(l+1)}} \frac{\hbar^2}{2m_e} \int d\mathbf{r} \phi_k \varphi_n (R_t + d) \frac{1 + \kappa_k |\mathbf{r} - \mathbf{a}|}{|\mathbf{r} - \mathbf{a}|^2} h_l^{(1)}(kr) \frac{\partial}{\partial \phi} Y_{lm}(\hat{\mathbf{r}}) \\ & - \frac{e}{\sqrt{l(l+1)}} \frac{\hbar^2}{2m_e} \int d\mathbf{r} \phi_k \varphi_n a_x \frac{1 + \kappa_k |\mathbf{r} - \mathbf{a}|}{|\mathbf{r} - \mathbf{a}|^2} h_l^{(1)}(kr) \\ & \times (\sin \phi \frac{\partial}{\partial \theta} Y_{lm}(\hat{\mathbf{r}}) + \frac{\cos \theta}{\sin \theta} \cos \phi \frac{\partial}{\partial \phi} Y_{lm}(\hat{\mathbf{r}})) \\ & - \frac{e}{\sqrt{l(l+1)}} \frac{\hbar^2}{2m_e} \int d\mathbf{r} \phi_k \varphi_n a_y \frac{1 + \kappa_k |\mathbf{r} - \mathbf{a}|}{|\mathbf{r} - \mathbf{a}|^2} h_l^{(1)}(kr) \\ & \times (-\cos \phi \frac{\partial}{\partial \theta} Y_{lm}(\hat{\mathbf{r}}) + \frac{\cos \theta}{\sin \theta} \sin \phi \frac{\partial}{\partial \phi} Y_{lm}(\hat{\mathbf{r}})). \end{aligned} \quad (11)$$

The transition probability as a function of displacement is presented in Fig. 4. Here we assume  $a_x = a_y$  for simplicity and set the parameters to  $d = 0.5\text{nm}$ ,  $R_t = 0.5\text{nm}$ ,  $V_b = -11\text{V}$ . Fig. 4 show the impact of displacement on transition probability. We found that a small displacement does not affect the results by an order of magnitude compared to when the tip is directly above, i.e.  $a_x = a_y = 0$ . There is a small rise here at the beginning because when the tip is directly above, only the spherical harmonics corresponding to the magnetic quantum number  $m = 0$  contribute, and when the tip deviates from directly above, all spherical harmonics contribute.

- 
- [1] C. J. Chen, *Phys. Rev. B* **42**, 8841 (1990).  
[2] J. Tersoff and D. R. Hamann, *Phys. Rev. Lett.* **50**, 1998 (1983).  
[3] J. Tersoff and D. R. Hamann, *Phys. Rev. B* **31**, 805 (1985).  
[4] Y. Zhang, Y. Luo, Y. Zhang, Y.-J. Yu, Y.-M. Kuang, L. Zhang, Q.-S. Meng, Y. Luo, J.-L. Yang, Z.-C. Dong, and J. G. Hou, *Nature* **531**, 623 (2016).  
[5] Z. Lin, L. V. Zhigilei, and V. Celli, *Phys. Rev. B* **77**, 075133 (2008).

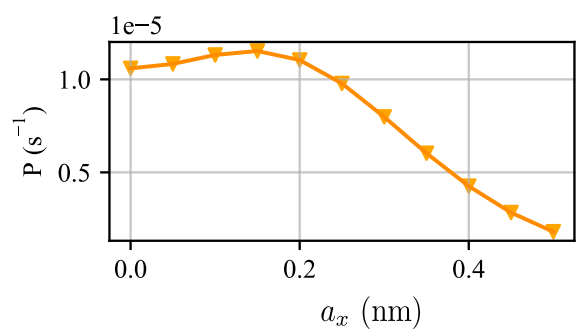

Figure 4. Transition probability when the tip center is displaced relative to the center of the atom.
